# Supplementary material for: Clock transition by continuous dynamical decoupling of a three-level system
Source: arXiv:1805.09435 ancillary file (2018-05-23)
Supplement: Supplementary file 1 [file clock_state_supplementary.pdf]

# Supplementary information for: Concatenated continuous dynamical decoupling of a three-level system

A. Stark,[1,2] N. Aharon,[3] A. Huck,[1] A. Retzker,[3] F. Jelezko,[2,4] and U.L. Andersen[1]

[1]*Department of Physics, Technical University of Denmark, Fysikvej, Kongens Lyngby 2800, Denmark*

[2]*Institute for Quantum Optics, Ulm University, Albert-Einstein-Allee 11, Ulm 89081, Germany*

[3]*Racah Institute of Physics, The Hebrew University of Jerusalem, Jerusalem 91904, Israel*

[4]*Center for Integrated Quantum Science and Technology ($IQ^{st}$), Ulm University, 89081 Germany*

## S1. SETUP CONFIGURATION

A standard home-build confocal microscope configuration was used to address individual NV centers. The sample, hosting the NVs, is a 98.9 % $^{12}$C electronic grade diamond substrate, with a 40 µm 99.8 % $^{12}$C low-N grade layer, grown by means of CVD. The top side of the diamond is attached to a glass slide with a lithographically deposed microwave structure, to enable close vicinity of the microwave field for an efficient microwave drive. The glass structure with the diamond was attached to a printed circuit board (PSB) sample holder with SMA connectors for microwave field delivery. The PSB board is mounted on a xyz home-build micrometer stage to position the sample relatively to the confocal scanner. The actual nanometer precise scanning operation in the confocal setup was realized by a xyz piezo scanner, P-527.3CD from Physik Instrumente with a E-725.3CD Digital Piezo Controller, which controls the position of an Olympus UPlanFL N 100X/1.30 ∞/0.17/FN 26.5 oil iris microscope objective.

The laser light is provided by a 2 W Verdi G2-SLM OPS 532 nm Laser diode, which is pulsed by an AOM from Brimrose. The red fluorescence is separated from the green illumination by a dichroic mirror FF552-Di02-25x36 from Semrock. The fluorescent response of the NV is converted with an avalanche photon diode (APD), SPCM-AQRH from Excelitas Technologies, into an electrical signal. The digitalized signal is either recorded by a custom configured XEM6310 LX45 FPGA from Opal Kelly, with a 950 MHz detection bandwidth (for fast counting), or with a PCI-6232 X-series card from National Instruments (for slow counting). The hardware triggered confocal scanning operation as well as the ODMR measurements are controlled with the NI PCI-6232 card.

The creation of the microwave field is either realized with a Rohde&Schwarz SMR20 microwave signal generator (for ODMR measurements) or with an arbitrary waveform generator AWG70002A from Tektronix (which was borrowed for a small period). In both cases, the microwave field was amplified by the ZHL-16W-43 S+ high power amplifier from Mini-Circuits.

All the instruments are remote controlled by a PC, which handles the measurement procedure and data acquisition. The powerful software suite Qudi [1] serves as the operational tool to establish the control over all hardware devices and perform all measurements.

The selected NV for this experiment was about one micrometer deep in the diamond and about 10 µm away from the microwave structure. The experiment was performed in the vicinity of the excited state level anti-crossing [2–4], where the nitrogen nuclear spin becomes polarized. Hence a static magnetic field of 358 G was applied to the NV center, aligned to its quantization axis.

Two neodymium magnet created the required quadrupole magnetic field. The magnets are attached (with a 3D printed holder) to a three axes NRT150/M 150 mm motorized linear translation stage with a BDC103 three channel controller from Thorlabs. In addition, a Thorlabs motorized rotation state with a TST001 driver controls the angular movement of the magnet.

A laser power of about 250 µW, measured before the objective, yields fluorescence counts of about 200 kcounts/s at zero magnetic bias fields.

## S2. SYSTEM PARAMETERS

### A. Pulsed ODMR measurements

A high resolution pulsed ODMR measurement was performed to identify potential coupling to adjacent $^{13}$C. Within the full width half maximum of the Lorentzian fit, no additional couplings to $^{13}$C are visible (cf. Fig. S1).

The average of both transition frequencies $\nu_1$ and $\nu_2$ should correspond to the zerofield splitting parameter $D = 2.87\,\mathrm{GHz}$. In the present case the average yields $(\nu_1 + \nu_2)/2 = (2870.7005 \pm 0.008)\,\mathrm{GHz}$ indicating a well aligned magnetic field.

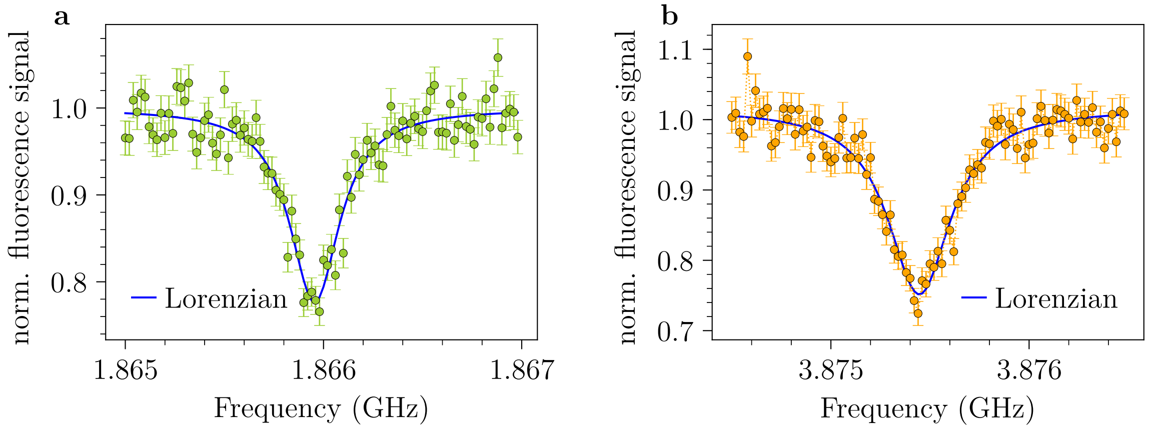


Figure S1. Pulsed ODMR measurement. (a) For the lower transition, a 3.3 µs long $\pi$-pulse was applied to invert the population. A Lorenzian fit yields an FWHM of $(306 \pm 23)\,\mathrm{kHz}$ at $\nu_1 = (1865.955 \pm 0.006)\,\mathrm{MHz}$. (b) For the upper transition, a 2.7 µs long $\pi$-pulse was applied, with an obtained FWHM of $(387 \pm 24)\,\mathrm{kHz}$ at $\nu_2 = (3875.446 \pm 0.006)\,\mathrm{MHz}$. The error bar in both plots corresponds to the normalized Poissonian error of the photon count signal.

### B. Coherence times of the Rabi drives

The drive between the transitions, $\nu_1$ and $\nu_2$, has to be adjusted to ensure the same Rabi frequency, $\Omega$. The inset of Fig. S2 shows the dependency of the Rabi frequency with respect to the applied amplitude in the signal generator. It becomes apparent that the lower transition with $\nu_1$ requires a larger amplitude to perform equal to $\nu_2$. The reason for the imbalances can be manifold and are discussed in Sec. S3.

The largest coherence time at $\nu_1$ was achieved for a drive of $\Omega/2\pi = (1.366 \pm 0.006)$ MHz with $T_2^{\Omega(\nu_1)} = (62 \pm 12)$ µ. For the upper transition at $\nu_2$ a drive of $\Omega/2\pi = (2.816 \pm 0.006)$ MHz yields $T_2^{\Omega(\nu_2)} = (159 \pm 24)$ µs.

An even larger different can be seen in the coherence times for both transitions. In order to record the coherence times, a first measurement determined the correct Rabi frequency for a given amplitude. Then the coherence time was measured by deliberately undersampling the obtained Rabi frequency to reduce considerable the measurement time.

There are interesting characteristics which can be extracted from the coherence time measurement in Fig. S2. Each driving field, $\Omega_i$, posses a noise component $\delta\Omega_i$. The amplitude of the driving noise is dependent on the strength of the drive and its scaling with amplitude is dependent on the measurement configuration. The coherence time curves coincide for small Rabi frequencies, as the external magnetic noise, $\delta B$, constitutes to be the main contribution. By increasing the drive a larger dressed state energy gap can be created protecting the system from the magnetic noise, $\delta B$. At the same time drive fluctuations become more prominent and dominate for a certain drive value the noise contribution. The sweet spot in the coherence time curve indicates a balanced situation, where the dressed states of the drive experiences similar noise contributions from the drive and the environment. Increasing the drive further leads to a non linear increase of the drive noise and the coherence time begins to decrease.

The drastic difference in the appearance of the coherence time curves indicates a frequency dependent noise of the drive fields for $\nu_1$ and $\nu_2$. In contrast to this, the magnetic noise seems to have an equal impact on both transitions,

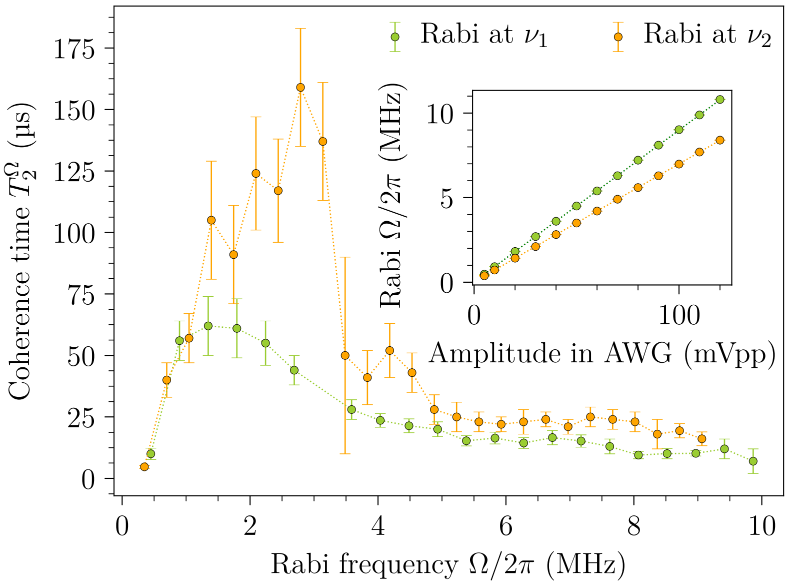


Figure S2. Rabi measurements at two transitions, $\nu_1 = (1864.942 \pm 0.019)$ MHz and at $\nu_2 = (3876.467 \pm 0.016)$ MHz. The main figure shows coherence times of Rabi oscillations, $T_2^\Omega$, as a function of Rabi drive, $\Omega$. The difference in $T_2^\Omega$ between both transitions originates mainly from a different drive noise characteristic at $\nu_1$ and $\nu_2$. The error bars are standard deviations, $\Delta T_2^\Omega$, from the fit $S(t) = A\cos(\Omega t)\exp\left(-t/T_2^\Omega\right)$ to the decaying Rabi signal. Inset: measurement of the Rabi frequency for different amplitudes of the signal generator. A linear fit to the slope yields $m_{\nu_1} = (89.68 \pm 0.10)$ kHz/mV and $m_{\nu_2} = (69.72 \pm 0.05)$ kHz/mV. The error bars correspond to $\Delta\Omega$.

which will be presented in the following sections.

### C. Ramsey measurements

A free induction decay or Ramsey measurement was performed on both transitions to identify that external and internal magnetic noise has the same impact on the $m_s = -1$ and $m_s = +1$ spin state. Fig. S3 illustrates that the average pure dephasing time, $T_2^* = (1.78 \pm 0.24)$ µs, corresponds well with the individual measurement.

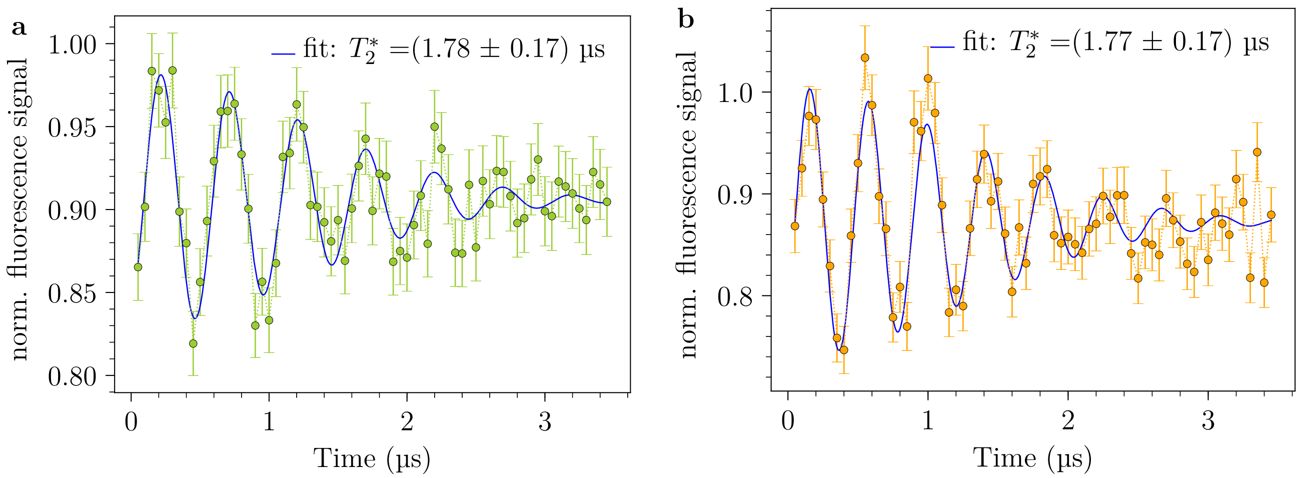


Figure S3. Ramsey coherence time measurement. The $\pi/2$ pulses in the scheme were deliberately detuned by 2 MHz to determine the coherence time, $T_2^*$, in the decreasing oscillating signal more accurately. The curves were fitted to the function $\propto \sin(\omega t + \phi)\exp\left\{-(t/T_2^*)^\beta\right\}$, where $\beta = 2.0 \pm 0.1$ was obtained for both curves. Hence, Gaussian uncorrelated noise can be assumed. (a) shows the lower transition and (b) the upper one, where both were measured at the ODMR frequency (+2 MHz) given in Fig. S1. The error bar in both plots corresponds to the normalized Poissonian error of the photon count signal.

### D. Hahn Echo measurements

A coherence time measurement with a standard Hahn Echo scheme was performed (cf. Fig. S4). Within the error bar, both transitions yield the same coherence time results. An averaged coherence time of $T_2 = (215 \pm 31)$ µs can be stated for the system, which coincides well with the individual measurement. Hence, the magnetic noise acting on the $m_s = -1$ and $m_s = +1$ can be considered as equal.

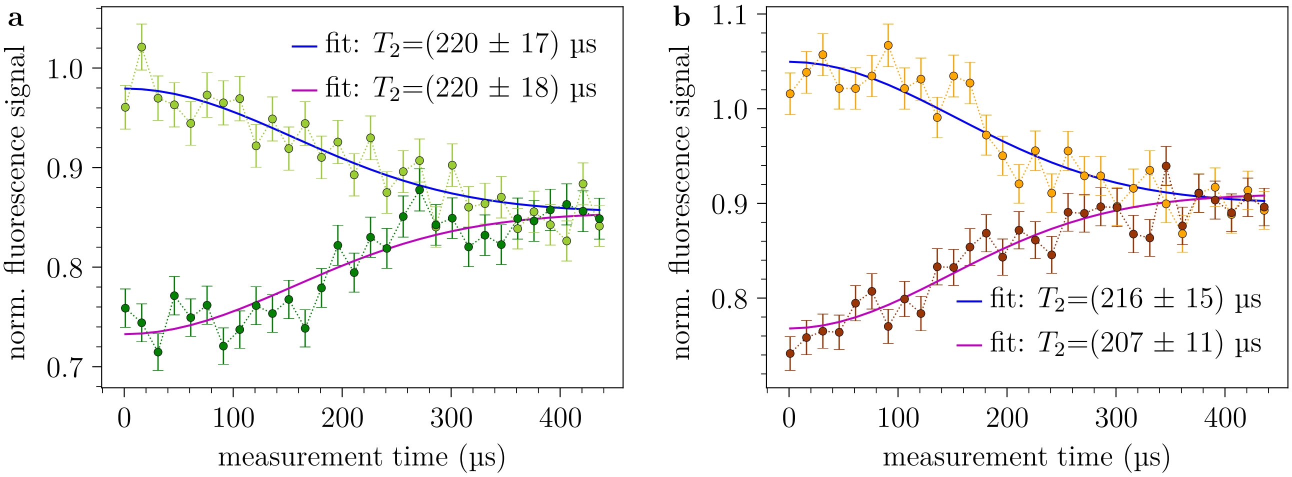


Figure S4. Hahn Echo coherence time measurement. The last pulse in the Hahn Echo measurement was either projecting the measurement to the bright ($\pi/2$-pulse, top curve) or to the dark ($3\pi/2$-pulse, lower curve) spin state of the NV center. Identifying the decoherence level to which both curves decaying to, increases the accuracy of the fit. The coherence time was obtained by fitting to $\propto \exp\{-(t/T_2)^2\}$ for (a) the lower and (b) the upper transition, corresponding to the ODMR measurement in Fig. S1. The error bar in both plots represent the normalized Poissonian error of the photon count signal.

## S3. ESTIMATED NOISE CHARACTERISTICS

In this section, we try to identify the components contributing to drive noise of the fields. From the Ramsey and the Hahn Echo measurements we can assume the same external magnetic noise at both transition frequencies, $\nu_1$ and $\nu_2$. In continuous dynamical decoupling the NV is permanently subjected to strong drive fields. Therefore, drive noise will be the strongest noise contribution in the scheme. As we did not had the possibility to measure the fast noise components directly with a fast oscilloscope, we would like to state the various noise contributions in our system, based on conservative estimates.

The drivings field in this work are created by the Tektronix AWG70002A. The maximal output amplitude for this device is 0.5 Vpp (or 1 Vpp by including the inverted channel) with a DAC accuracy of 8bit, yielding a maximum precision of $0.5\,\text{Vpp}/2^8 \approx 2\,\text{mVpp}$ or 1 mV for the amplitude of an oscillating signal. Consequently, a sinusoidal field with amplitude of 0.25 V (0.5 Vpp) has an accuracy of $(250 \pm 1)$ mV, which gives a relative error of 0.78 %. The vendor specifies the amplitude accuracy to ±10 mVpp [5], which increases the relative error to 4 %, indicating that besides the DAC inaccuracy, other noise sources exist. Therefore, the application of 4 sinusoidal fields at different frequencies can have at maximum 1/4 of the total amplitude noise, if it is equally distributed on all of them (which is not necessarily the case). Thus, one frequency component is accurate up to $(62.5 \pm 1.3)$ mV, yielding an relative amplitude error of 2 %.

A field of 62.5 mV (= 125 mVpp) would create (see the inset of Fig.1 in the main text) a Rabi drive of the order of 10 MHz. Increasing the drive field above that value caused heating problems, as a lot of power is dissipated in the microwave structure causing a drastic decrease in ODMR contrast and fluorescence signal. To prevent that from

happening the amplitude has to be lowered so that such effects are not dominating. We found a balance between the thermal effects and the maximal obtainable Rabi frequency for fields of the order of 40 mVpp, if 4 fields are used simultaneously (which result in a total amplitude of 160 mVpp). Given these limitation in the drive fields, the relative noise for each frequency components is on average 6.25 %.

Moreover, the amplitude noise of the AWG is correlated to its base clock, which introduces correlated (amplitude) noise on µs timescale and may very well be responsible for frequency dependent (fast) noise imbalances, translated to the dressed states of the considered three-level system (see main text Fig. 4). The origin of this noise character can be grasp by investigating how data become sampled in an AWG.

Modern, very fast AWGs (with sample rate exceeding 1GS/s) do not process each sample directly as the rate the data is read exceeds the speed of common semiconductor memories [6]. To circumvent the problem, data is processed in parallel and then multiplexed inside the high-speed digital logic in the AWG that drives the DAC. However, the multiplexing operation is directly bound to the internal clock of the AWG, which is usually of the order of 10MHz and thus, creates correlation on that time base. Any errors in the timing of the internal clock edge translate directly into timing errors in the analog output, which reflects to phase noise and is immediately detectable by amplitude fluctuations. This is a noise source, which adds to the DAC inaccuracy and creates (among other effects) the total noise floor of the device. Eventually, a high-speed oscilloscope would be the preferential choice to identify fast noise on the frequency components.

On top of this, we assume also a frequency dependent noise, since the output of the amplifier is not flat over a range of $\nu_2 - \nu_1 \approx 2\,\mathrm{GHz}$. Moreover, the microwave structure experiences frequency dependent attenuation of the applied drive fields leading (among other contributions) to different Rabi frequencies for $\nu_1$ and $\nu_2$ at the same amplitude output (cf. the inset of Fig.1 in the main text).

All these various noise contributions have a strong impact on the drive of the NV system as they cause the dressed states to fluctuate. Therefore it becomes a crucial task in CCD to reduce the impact of noise, introduced by multi-frequency drive fields, by creating robust states, which suffer less from drive noise contributions. By demonstrating robustness to all these noise sources underlines the importance of the present work.


[1] J. M. Binder, A. Stark, N. Tomek, J. Scheuer, F. Frank, K. D. Jahnke, C. Müller, S. Schmitt, M. H. Metsch, T. Unden, T. Gehring, A. Huck, U. L. Andersen, L. J. Rogers, and F. Jelezko, SoftwareX **6**, 85 (2017).

[2] V. Jacques, P. Neumann, J. Beck, M. Markham, D. Twitchen, J. Meijer, F. Kaiser, G. Balasubramanian, F. Jelezko, and J. Wrachtrup, Physical Review Letters **102**, 057403 (2009).

[3] V. Ivády, K. Szász, A. L. Falk, P. V. Klimov, D. J. Christle, E. Janzén, I. A. Abrikosov, D. D. Awschalom, and A. Gali, Physical Review B **92**, 115206 (2015).

[4] D. A. Broadway, J. D. Wood, L. T. Hall, A. Stacey, M. Markham, D. A. Simpson, J.-P. Tetienne, and L. C. Hollenberg, Physical Review Applied **6**, 064001 (2016).

[5] Tektronix, "AWG70000a Arbitrary Waveform Generator Datasheet | Tektronix," (2016).

[6] Keysight Technologies, "The ABC's of Arbitrary Waveform Generation - An Application Note," (2006).
